# Supplementary material for: Calibrated Selective Classification
Source: arXiv:2208.12084 source file (2024-06-20)
Supplement: Supplementary file 1 [file evaluation.tex]

\section{Empirically evaluating calibration}
\label{app:evaluation}
