# Supplementary material for: Calibrated Selective Classification
Source: arXiv:2208.12084 source file (2024-06-20)
Supplement: Supplementary file 2 [file other_calibration.tex]

\section{Alternative approaches to calibration}
\label{app:calibration_defs}
